# Supplementary material for: Text Classification via Large Language Models
Source: arXiv:2305.08377 source file (2023-10-09)
Supplement: Supplementary file 1 [file appendix_dataset_statistic.tex]

\begin{table*}[h]
  \centering
  \small
  \scalebox{0.68}{
  \begin{tabular}{lccccccc}\toprule
    & \multicolumn{3}{c}{{\it Non-Semantic Shift (NSS) Datasets}} & \multicolumn{4}{c}{{\it Semantic Shift (SS) Datasets}}\\
    \cmidrule(r){2-4}\cmidrule(r){5-8}\\
    & {\bf 20News-6S} & {\bf AG-EXT} & {\bf Yahoo-AG-five} & {\bf Reuters-$m$K-$n$L} & {\bf AG-FL} & {\bf AG-FM} & {\bf Yahoo-FM}\\\midrule
    {\it Adapted From} & 20News & AGNews\&AGCorpus & Yahoo\&AGCorpus & Reuters & AGNews\&AGCorpus & AGNews\&AGCorpus & Yahoo \\ 
    \specialrule{0em}{1pt}{1pt}
    \cdashline{1-8}
    \specialrule{0em}{1pt}{1pt}
    {\it \# Labels in T} & 6 & 4 & 5 & $m$ & 4 & 4 & 5 \\ 
    {\it \# Instances in T} & 8,283 & 112,400 & 675,000 & $f(m,\text{train})$ & 116,000 & 116,000 & 680,000 \\ 
    \specialrule{0em}{1pt}{1pt}
    \cdashline{1-8}
    \specialrule{0em}{1pt}{1pt}
    {\it \# Labels in ID-V} & 6 & 4 & 5 & $m$ & 4 & 4 & 5 \\ 
    {\it \# Instances in ID-V} & 1,034 & 7,600 & 25,000 & $f(m,\text{valid})$ & 4,000 & 4,000 & 20,000 \\ 
    {\it \# Labels in OOD-V} & 6 & 4 & 5 & $n$ & 4 & 4 & 5 \\ 
    {\it \# Instances in OOD-V} & 846 & 7,600 & 25,000 & $f(n,\text{valid})$ & 4,000 & 4,000 & 20,000 \\ 
    \specialrule{0em}{1pt}{1pt}
    \cdashline{1-8}
    \specialrule{0em}{1pt}{1pt}
    {\it \# Labels in ID-T} & 6 & 4 & 5 & $m$ & 4 & 4 & 5 \\ 
    {\it \# Instances in ID-T} & 1,034 & 7,600 & 25,000 & $f(m,\text{test})$ & 4,000 & 4,000 & 25,000 \\ 
    {\it \# Labels in OOD-T} & 6 & 4 & 5 & $n$ & 4 & 4 & 5 \\ 
    {\it \# Instances in OOD-T} & 846 & 7,600 & 25,000 & $f(n,\text{test})$ & 4,000 & 4,000 & 25,000 \\\bottomrule
  \end{tabular}
  }
  \caption{Example table 1.}
  \label{tab:benchmark}
\end{table*}
