# Supplementary material for: Text Classification via Large Language Models
Source: arXiv:2305.08377 source file (2023-10-09)
Supplement: Supplementary file 2 [file appendix_lowresource_dataset.tex]

\begin{table*}[t]
\center
\small
\begin{tabular}{l|lcc|ccc|c}\hline
{\bf Dataset}  & {\bf Task}& {\bf \# Label} & {\bf Source} & {\bf \# Train} & {\bf \# Dev} & {\bf \# Test} & {\bf Length Avg}\\\hline
SST-2 & sentiment & 2 & &  & 872 & 1,821 &  \\
AGNews & topic & 4 & &  & 24,000 & 7,600 &  \\
R8 & & topic8 & &  & 544 & 2,189 & \\
R52 & & 52 &  & 5,905 & 627 & 2,568 &  \\
MR & sentiment & 2 & & 6,398 & 710 & 3,554 &  \\\hline
\end{tabular}
\caption{Low-resource Dataset}
\label{appendix:dataset}
\end{table*}
